# Supplementary material for: Revealing Domain-Spatiality Patterns for Configuration Tuning: Domain Knowledge Meets Fitness Landscapes
Source: arXiv:2603.19897 source file (2026-03-23)
Supplement: Supplementary file 1 [file supp.tex]

The workloads we studied are diverse and domain-specific. Each workload is selected to reflect realistic usage scenarios for its corresponding system:
\begin{itemize}
    \item \textbf{\textsc{Jump3r}} encodes raw \texttt{WAVE} audio signals to MP3, with variations in file size, signal length, sampling rate, and number of channels.
    \item \textbf{\textsc{X264}} encodes raw video frames (y4m format) across different resolutions (low/DS up to 4K) and file sizes.
    \item \textbf{\textsc{Kanzi}, \textsc{Xz}, and \textsc{Lrzip}} Compress mixed-type files (text, binary, structured data, etc) or single-type files from community benchmarks.  Additionally, custom datasets, including the Hubble Deepfield image and a Linux kernel binary, are used to augment the workloads. For \textsc{Xz} and \textsc{Lrzip}, different parameterizations of UIQ2 benchmark\footnote{\url{http://mattmahoney.net/dc/uiq/}} are added to study the effect of varying file size. 
    \item \textbf{\textsc{Z3}} evaluates the satisfiability of logical problems in SMT2 format. The workload consists of the six longest-running instances from Z3’s performance test suite, augmented with additional instances from the SMT2-Lib\footnote{\url{https://smt-comp.github.io/2017/benchmarks.html}} repository to increase diversity in logic types.
    \item \textbf{\textsc{Batik}} transforms \texttt{SVG} vector graphic into a bitmap. The workload consists of resources from the Wikimedia Commons collection\footnote{\url{https://commons.wikimedia.org/wiki/Category:Images}}, varying primarily in file size.
    \item \textbf{\textsc{H2}} executs database transactions using different \textsc{OLTPBench}~\cite{difallah2013oltp} benchmarks (\texttt{Voter}, \texttt{SmallBank}, \texttt{TPC-H}, \texttt{YCSB}). The scale factor is varied to adjust transaction complexity.
    \item \textbf{\textsc{Dconvert}} transforms resources (e.g., image files) at different scales. The workload includes various input formats (\texttt{JPEG}, \texttt{PNG}, \texttt{PSD}, \texttt{SVG}) with variations in file size.
\end{itemize}

\subsection{Landscape Metrics}
To systematically investigate the characteristics of systems, we analyze both landscape metrics and domain-specific factors, integrating empirical FLA observations with system's domain knowledge. Specifically, we evaluate landscape structures using the key metrics introduced in Section \ref{subsection: Landscape Metrics}.

\miqing{I am wondering if we could use the three major features (ruggedness level, local structure and global structure) that SE people understand better to structure this section.}

\subsubsection{Distance Measures and Neighborhood}
\label{subsection:neighbor_setup}
As introduced in Section \ref{subsection:distance_measures_and_neighborhood}, the neighborhood of a configuration is typically defined by a Hamming distance of $d(\boldsymbol{c}^{\prime}, \boldsymbol{c})=1$, where neighbors differ by a single configuration option. However, the datasets used in this study are constructed by sampling rather than via exhaustive grid search~\cite{muhlbauer2023analyzing}, this strict definition can leave many configurations without neighbors, especially in sparse regions. To address this, we adaptively adjust the neighborhood radius to ensure that the average number of neighbors for configurations is at least $\frac{n}{2}$, where $n$ is the configuration dimensionality. This balances sampling sparsity with meaningful connectivity, preserving landscape structure for robust topological analysis.

\subsubsection{Fitness Distance Correlation}

FDC ($\varrho$) measures the correlation between performance and distance to the global optimum, capturing the overall searchability of the landscape. A strong correlation ($\varrho$ $\geq$ 0.15) suggests a globally guided search, whereas weak correlation ($\mathcal{-}0.15 \textless \varrho \textless 0.15$) and negative correlation ($\varrho \leq \mathcal{-} 0.15$) indicate irregular and deceptive structures, respectively, increasing the challenge of optimization~\cite{jones1995fitness}.

\subsubsection{Basin of Attraction}

%Basin of attraction refers to the search regions leading directly to the local optima during a local search. Here, the local search follows the neighborhood structure defined in Section \ref{subsection:neighbor_setup}, with a step size equal to the defined neighborhood distance. If neighbors differ by $d$ options, the local search perturbs exactly $d$ options per step, ensuring consistency in identifying basin of attraction. The basin size of a local optimum reflects how many configurations are drawn into it. The basin size of the global optimum, on the other hand, , provides insights into its accessibility---larger basin size indicate that more configurations naturally converge to the global optimum, making it easier to reach, whereas smaller ones suggests a more fragmented landscape, hindering direct convergence.

Basin of attraction of a (local) optimal point refers to the set of all possible starting points in the search space that, when using a local search algorithm, will eventually converge to that specific optimal point. Here, we consider hill climbing as the local search algorithm, and its step size follows the neighborhood structure defined in Section \ref{subsection:neighbor_setup}. In other words, if neighbors differ by $d$ options, the local search needs to take $d$ options per step, ensuring consistency in identifying basin of attraction. Clearly, a larger attraction basin size indicates that more configurations naturally converge to the optimum, making it easier to reach, whereas a smaller one suggests a more fragmented landscape. Here, we regard the basin size larger than $21\%$ (against the whole search space) as an ``easy'' problem, given the fact that randomly sampling $20$ configurations (same as many population-based search in software configuration tuning \cite{chen2024mmo,DBLP:journals/corr/abs-2501-00840}) for local search will lead to a probability of $99\%$ of locating at least one optimum in the search space (i.e., $1-(1-0.99)^{1/20}\approx0.21$).

\subsubsection{Local Optima}    
Local optima characterize the modality of a landscape. A higher number of local optima indicates a more complex landscape, making it more challenging to navigate towards the global optimum. The quality distribution of these local optima shapes search behaviors---poor local optima would increase the risk of premature stagnation, while high-quality ones allow to yield competitive solutions despite not converging to the absolute best configuration. Here, we classify the quality of local optima into three tiers based on the relative quality metric $\ell_q$: high-quality ($\ell_q\geq0.67$); medium quality ($0.33 \textless \ell_q \textless 0.67 $); and low quality ($\ell_q \leq 0.33$).

\subsubsection{Autocorrelation}

Autocorrelation ($r$) quantifies landscape ruggedness by measuring performance similarity across neighboring configurations visited during random walks through the landscape. To accommodate analysis on sampled datasets, our random walk starts with a step size of $d$ = 1. If no neighbor is found, $d$ is incrementally increased until a valid neighbor is located, ensuring continuity. The walk proceeds until all configurations in the dataset are visited, recording the total walk length $N$. Finally, autocorrelation is computed using Equation (\ref{eq:autocorrelation}). A high autocorrelation ($r \geq 0.5$) suggests a smoother landscape; Moderate autocorrelation ($0.2 \textless r \textless 0.5$) indicates medium ruggedness; And low autocorrelation ($r \leq 0.2$) suggests a highly rugged landscape with sharp performance fluctuations~\cite{stadler1996landscapes,weinberger1990correlated,huang2024rethinking}.
